# Supplementary material for: A Density-Based Basis-Set Incompleteness Correction for GW Methods
Source: arXiv:1910.12238 source file (2020-01-04)
Supplement: Supplementary file 1 [file GW-srDFT-SI.pdf]

# Supplementary Materials for "A Density-Based Basis-Set Incompleteness Correction for GW Methods"

Pierre-François Loos,[1,a)] Barthélémy Pradines,[2,3] Anthony Scemama,[1] Emmanuel Giner,[2] and Julien Toulouse[2,4,b)]
[1)] *Laboratoire de Chimie et Physique Quantiques (UMR 5626), Université de Toulouse, CNRS, UPS, France*
[2)] *Laboratoire de Chimie Théorique (UMR 7616), Sorbonne Université, CNRS, Paris, France*
[3)] *Institut des Sciences du Calcul et des Données, Sorbonne Université, Paris, France*
[4)] *Institut Universitaire de France, Paris, France*

## I. COMPLEMENTARY SHORT-RANGE CORRELATION POTENTIALS

Here, we provide the expressions of the complementary short-range LDA and PBE correlation potentials used in the present work in the case of closed-shell systems.

### A. Complementary short-range LDA correlation potential

The complementary short-range LDA correlation energy functional with multideterminant reference has the expression[1,2]

$$\bar{E}^{\mathcal{B}}_{\text{srLDA}}[n] = \int n(\mathbf{r})\bar{\varepsilon}^{\text{srLDA}}_{\text{c,md}}(n(\mathbf{r}),\mu^{\mathcal{B}}(\mathbf{r}))d\mathbf{r}, \tag{1}$$

with

$$\bar{\varepsilon}^{\text{srLDA}}_{\text{c,md}}(n,\mu) = \bar{\varepsilon}^{\text{srLDA}}_{\text{c}}(n,\mu) + \Delta^{\text{lr-sr}}(n,\mu), \tag{2}$$

where $\bar{\varepsilon}^{\text{srLDA}}_{\text{c,md}}(n,\mu)$ is the complementary short-range LDA correlation energy functional (with single-determinant reference) and $\Delta^{\text{lr-sr}}(n,\mu)$ is a mixed long-range/short-range contribution, both parametrized in Ref. 2.

The corresponding complementary srLDA potential is

$$\begin{aligned}\bar{v}^{\mathcal{B}}_{\text{srLDA}}[n](\mathbf{r}) &= \frac{\delta \bar{E}^{\mathcal{B}}_{\text{srLDA}}[n]}{\delta n(\mathbf{r})} \\ &= \bar{\varepsilon}^{\text{srLDA}}_{\text{c,md}}(n(\mathbf{r}),\mu^{\mathcal{B}}(\mathbf{r})) \\ &\quad + n(\mathbf{r})\frac{\partial \bar{\varepsilon}^{\text{srLDA}}_{\text{c,md}}}{\partial n}(n(\mathbf{r}),\mu^{\mathcal{B}}(\mathbf{r})).\end{aligned} \tag{3}$$

The density derivative of $\bar{\varepsilon}^{\text{srLDA}}_{\text{c,md}}$ is calculated as

$$\frac{\partial \bar{\varepsilon}^{\text{srLDA}}_{\text{c,md}}}{\partial n} = \frac{\partial \bar{\varepsilon}^{\text{srLDA}}_{\text{c}}}{\partial n} + \frac{\partial \Delta^{\text{lr-sr}}}{\partial n}, \tag{4}$$

where $\partial \bar{\varepsilon}^{\text{srLDA}}_{\text{c}}/\partial n$ is given as a subroutine on Paola Gori-Giorgi's website (https://www.quantummatter.eu/source-codes-2) and we have calculated $\partial \Delta^{\text{lr-sr}}/\partial n$ by taking the derivative of Eq. (42) of Ref. 2.

### B. Complementary short-range PBE correlation potential

The complementary short-range PBE correlation energy functional with multideterminant reference has the expression[3]

$$\bar{E}^{\mathcal{B}}_{\text{srPBE}}[n] = \int n(\mathbf{r})\bar{\varepsilon}^{\text{sr,PBE}}_{\text{c,md}}(n(\mathbf{r}),s(\mathbf{r}),\mu^{\mathcal{B}}(\mathbf{r}))d\mathbf{r}, \tag{5}$$

with

$$\bar{\varepsilon}^{\text{sr,PBE}}_{\text{c,md}}(n,s,\mu) = \frac{\varepsilon^{\text{PBE}}_{\text{c}}(n,s)}{1+\beta(n,s)\mu^3}. \tag{6}$$

Here, $\varepsilon^{\text{PBE}}_{\text{c}}(n,s)$ is the usual PBE correlation functional,[4] $s$ is the reduced density gradient,

$$\beta(n,s) = \frac{3}{2\sqrt{\pi}(1-\sqrt{2})}\frac{\varepsilon^{\text{PBE}}_{\text{c}}(n,s)}{n^{\text{UEG}}_2(n)/n}, \tag{7}$$

and

$$n^{\text{UEG}}_2(n) = n^2 g_0(r_s) \tag{8}$$

is the on-top pair density of the uniform electron gas (UEG). In Eq. (8), $g_0(r_s)$ is the UEG on-top pair-distribution function written as a function of the Wigner-Seitz radius $r_s = (4\pi n/3)^{-1/3}$. We use the parametrization of $g_0(r_s)$ given in Eq. (46) of Ref. 5.

The corresponding complementary srPBE potential is

$$\begin{aligned}\bar{v}^{\mathcal{B}}_{\text{srPBE}}[n](\mathbf{r}) &= \frac{\delta \bar{E}^{\mathcal{B}}_{\text{srPBE}}[n]}{\delta n(\mathbf{r})} \\ &= \bar{\varepsilon}^{\text{sr,PBE}}_{\text{c,md}}(n(\mathbf{r}),s(\mathbf{r}),\mu^{\mathcal{B}}(\mathbf{r})) \\ &\quad + n(\mathbf{r})\frac{\partial \bar{\varepsilon}^{\text{sr,PBE}}_{\text{c,md}}}{\partial n} \\ &\quad - \nabla\cdot\left(n(\mathbf{r})\frac{\partial \bar{\varepsilon}^{\text{sr,PBE}}_{\text{c,md}}}{\partial \nabla n}\right).\end{aligned} \tag{9}$$

Hence, we have to compute the density derivative $\partial \bar{\varepsilon}^{\text{sr,PBE}}_{\text{c,md}}/\partial n$ and the density-gradient derivative $\partial \bar{\varepsilon}^{\text{sr,PBE}}_{\text{c,md}}/\partial \nabla n$.

#### 1. *Density derivative*

From Eq. (6), the density derivative is found to be

$$\frac{\partial \bar{\varepsilon}^{\text{sr,PBE}}_{\text{c,md}}}{\partial n} = \frac{1}{1+\beta\mu^3}\frac{\partial \varepsilon^{\text{PBE}}_{\text{c}}}{\partial n} - \frac{\varepsilon^{\text{PBE}}_{\text{c}}\mu^3}{(1+\beta\mu^3)^2}\frac{\partial \beta}{\partial n}, \tag{10}$$

a)Corresponding author: loos@irsamc.ups-tlse.fr
b)Corresponding author: toulouse@lct.jussieu.fr

where $\partial\varepsilon_c^{PBE}/\partial n$ is the density derivative of the usual PBE correlation functional, and

$$\frac{\partial\beta}{\partial n} = \frac{3}{2\sqrt{\pi}(1-\sqrt{2})}\left[\frac{1}{n_2^{UEG}/n}\frac{\partial\varepsilon_c^{PBE}}{\partial n} - \frac{\varepsilon_c^{PBE}}{(n_2^{UEG}/n)^2}\frac{\partial(n_2^{UEG}/n)}{\partial n}\right]. \quad (11)$$

The only remaining missing part is the derivative of $n_2^{UEG}/n$ which is

$$\frac{\partial(n_2^{UEG}/n)}{\partial n} = \frac{\partial[n g_0(r_s)]}{\partial n} = g_0(r_s) + n\frac{\partial g_0(r_s)}{\partial n}, \quad (12)$$

with

$$\frac{\partial g_0(r_s)}{\partial n} = \frac{\partial r_s}{\partial n}\frac{\partial g_0(r_s)}{\partial r_s} = -(6n^2\sqrt{\pi})^{-2/3}\frac{\partial g_0(r_s)}{\partial r_s}. \quad (13)$$

Finally, we calculate $\partial g_0(r_s)/\partial r_s$ by taking the derivative of Eq. (46) of Ref. 5

$$\frac{\partial g_0(r_s)}{\partial r_s} = \frac{e^{-F r_s}}{2}\big[(-B + 2Cr_s + 3Dr_s^2 + 4Er_s^3) - F(1 - Br_s + Cr_s^2 + Dr_s^3 + Er_s^4)\big], \quad (14)$$

with $C = 0.0819306$, $F = 0.752411$, $D = -0.0127713$, $E = 0.00185898$, and $B = 0.7317 - F$.

### 2. *Density-gradient derivative*

For the density-gradient derivative, we use the chain rule

$$\frac{\partial\bar{\varepsilon}_{c,md}^{sr,PBE}}{\partial\nabla n} = \frac{\partial\bar{\varepsilon}_{c,md}^{sr,PBE}}{\partial\varepsilon_c^{PBE}}\frac{\partial\varepsilon_c^{PBE}}{\partial\nabla n}, \quad (15)$$

where $\partial\varepsilon_c^{PBE}/\partial\nabla n$ is the density-gradient derivative of the usual PBE correlation functional, and

$$\frac{\partial\bar{\varepsilon}_{c,md}^{sr,PBE}}{\partial\varepsilon_c^{PBE}} = \frac{1}{1+\beta\mu^3} - \frac{\varepsilon_c^{PBE}\mu^3}{(1+\beta\mu^3)^2}\frac{\partial\beta}{\partial\varepsilon_c^{PBE}}, \quad (16)$$

with

$$\frac{\partial\beta}{\partial\varepsilon_c^{PBE}} = \frac{3}{2\sqrt{\pi}(1-\sqrt{2})}\frac{1}{n_2^{UEG}/n}. \quad (17)$$

## II. ADDITIONAL GRAPHS OF THE CONVERGENCE OF THE IPS OF THE GW20 SUBSET

Graphs reporting the convergence of the IPs of each molecule of the GW20 subset at the $G_0W_0$@HF and $G_0W_0$@PBE0 levels are given in Figs. 1 and 2, respectively.


[1] Toulouse, J.; Gori-Giorgi, P.; Savin, A. A Short-Range Correlation Energy Density Functional With Multi-Determinantal Reference. *Theor. Chem. Acc.* **2005**, *114*, 305.

[2] Paziani, S.; Moroni, S.; Gori-Giorgi, P.; Bachelet, G. B. Local-Spin-Density Functional For Multideterminant Density Functional Theory. *Phys. Rev. B* **2006**, *73*, 155111.

[3] Loos, P. F.; Pradines, B.; Scemama, A.; Toulouse, J.; Giner, E. A Density-Based Basis-Set Correction for Wave Function Theory. *J. Phys. Chem. Lett.* **2019**, *10*, 2931–2937.

[4] Perdew, J. P.; Burke, K.; Ernzerhof, M. Generalized Gradient Approximation Made Simple. *Phys. Rev. Lett.* **1996**, *77*, 3865–3868.

[5] Gori-Giorgi, P.; Savin, A. Properties Of Short-Range And Long-Range Correlation Energy Density Functionals From Electron-Electron Coalescence. *Phys. Rev. A* **2006**, *73*, 032506.

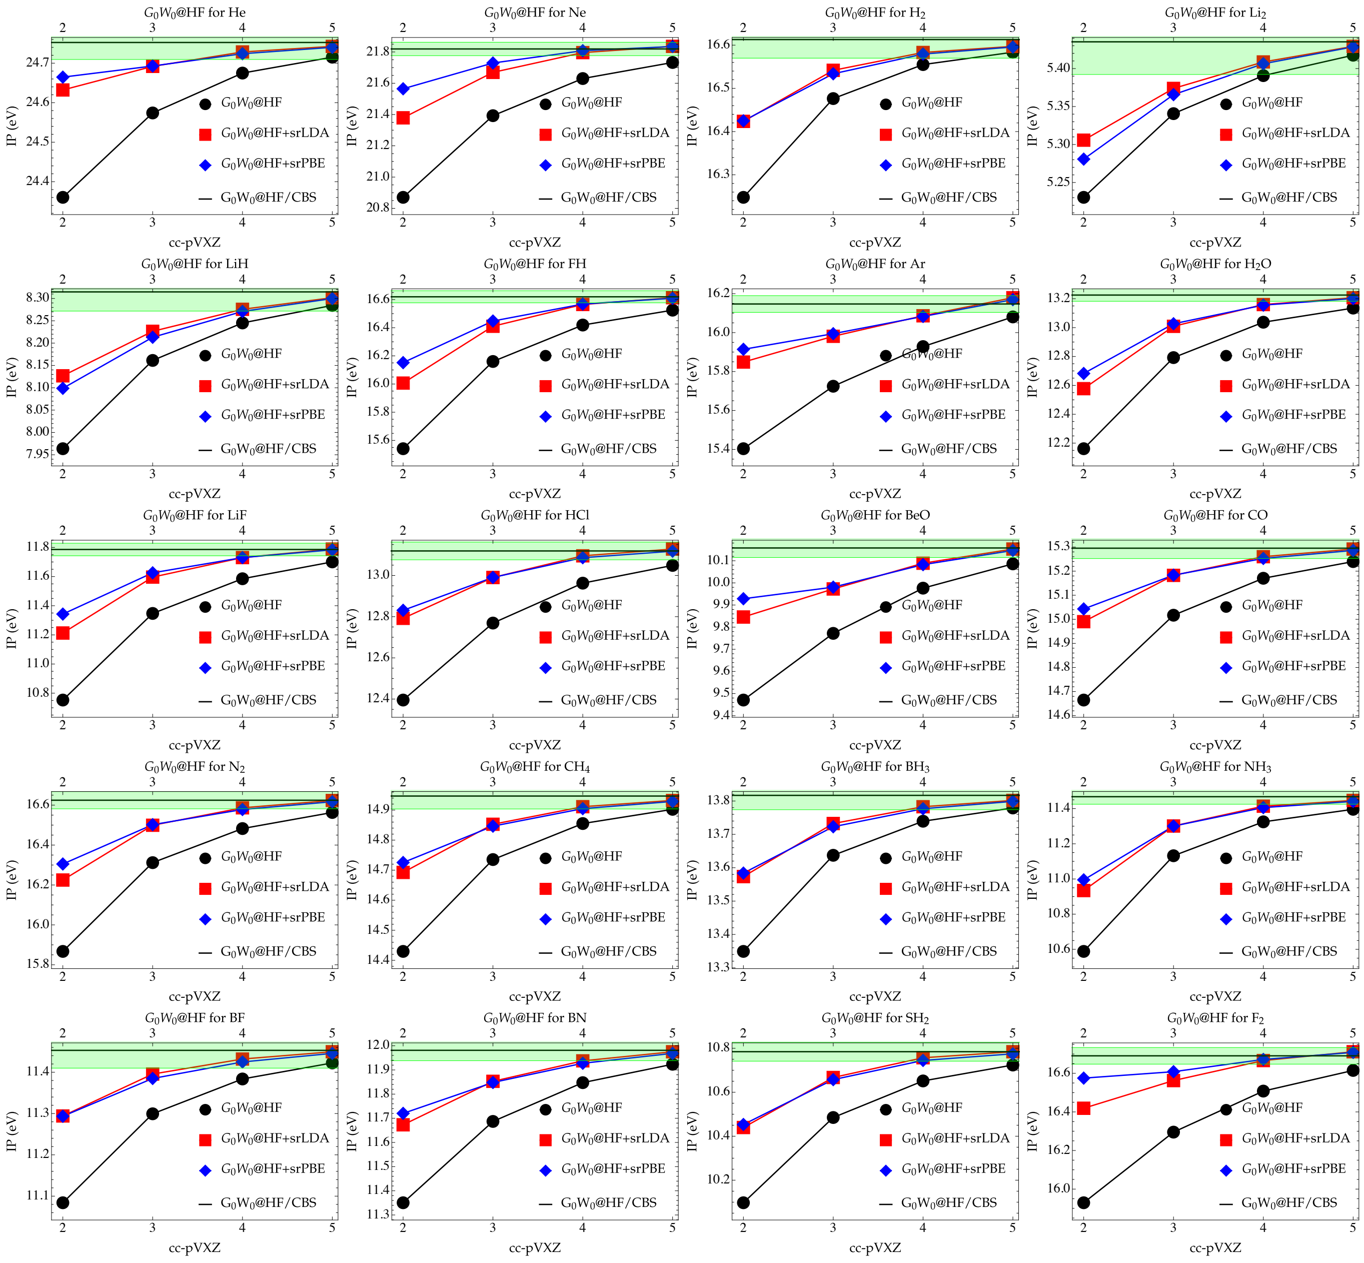


FIG. 1. IPs (in eV) computed at the $G_0W_0$@HF (black circles), $G_0W_0$@HF+srLDA (red squares), and $G_0W_0$@HF+srPBE (blue diamonds) levels of theory with increasingly large Dunning's basis sets (cc-pVDZ, cc-pVTZ, cc-pVQZ, and cc-pV5Z) for the 20 smallest molecules of the GW100 set. The thick black line represents the CBS value obtained by extrapolation with the three largest basis sets.

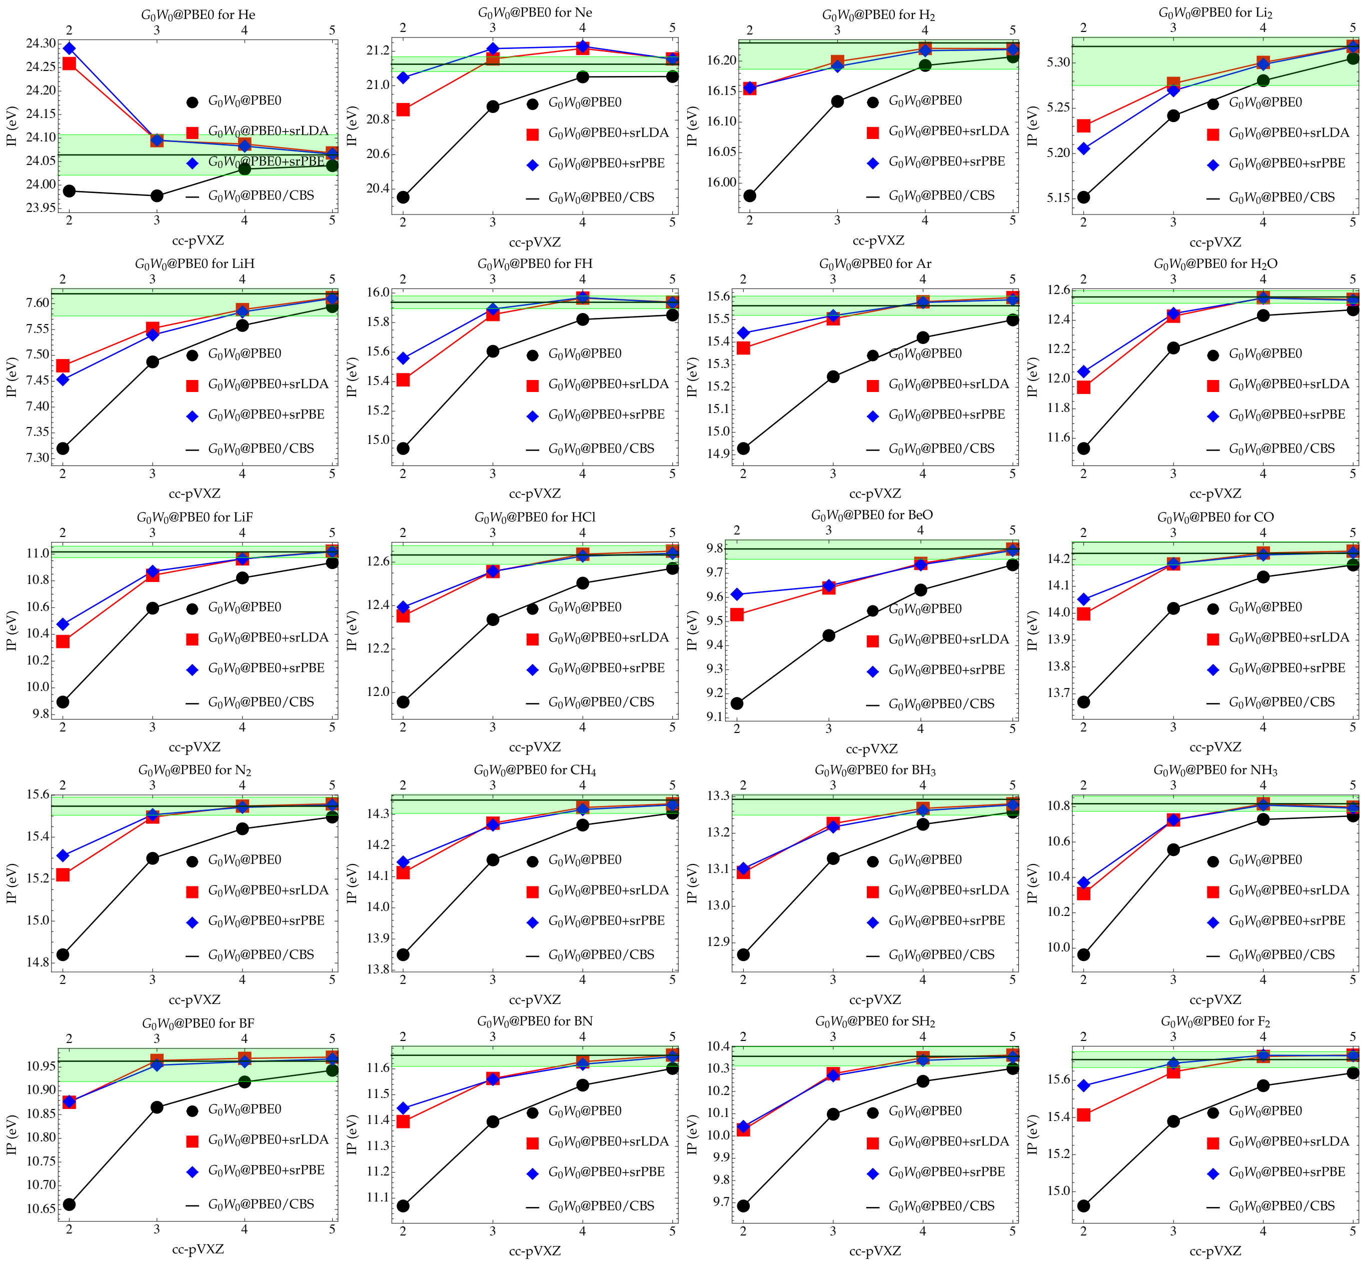


FIG. 2. IPs (in eV) computed at the $G_0W_0$@PBE0 (black circles), $G_0W_0$@PBE0+srLDA (red squares), and $G_0W_0$@PBE0+srPBE (blue diamonds) levels of theory with increasingly large Dunning's basis sets (cc-pVDZ, cc-pVTZ, cc-pVQZ, and cc-pV5Z) for the 20 smallest molecules of the GW100 set. The thick black line represents the CBS value obtained by extrapolation with the three largest basis sets.
